# Supplementary material for: Approximate Inference for Constructing Astronomical Catalogs from Images
Source: arXiv:1803.00113 source file (2019-04-10)
Supplement: Supplementary file 1 [file 9_experiment_supplement.tex]

\section*{Supplement B: Additional experimental results}
\label{experiment_plots}
This section presents more experimental results for the synthetic and Stripe 82 datasets.

%---- error plots on synthetic data -------
\begin{figure}
  \centering
  \includegraphics[width=\linewidth]{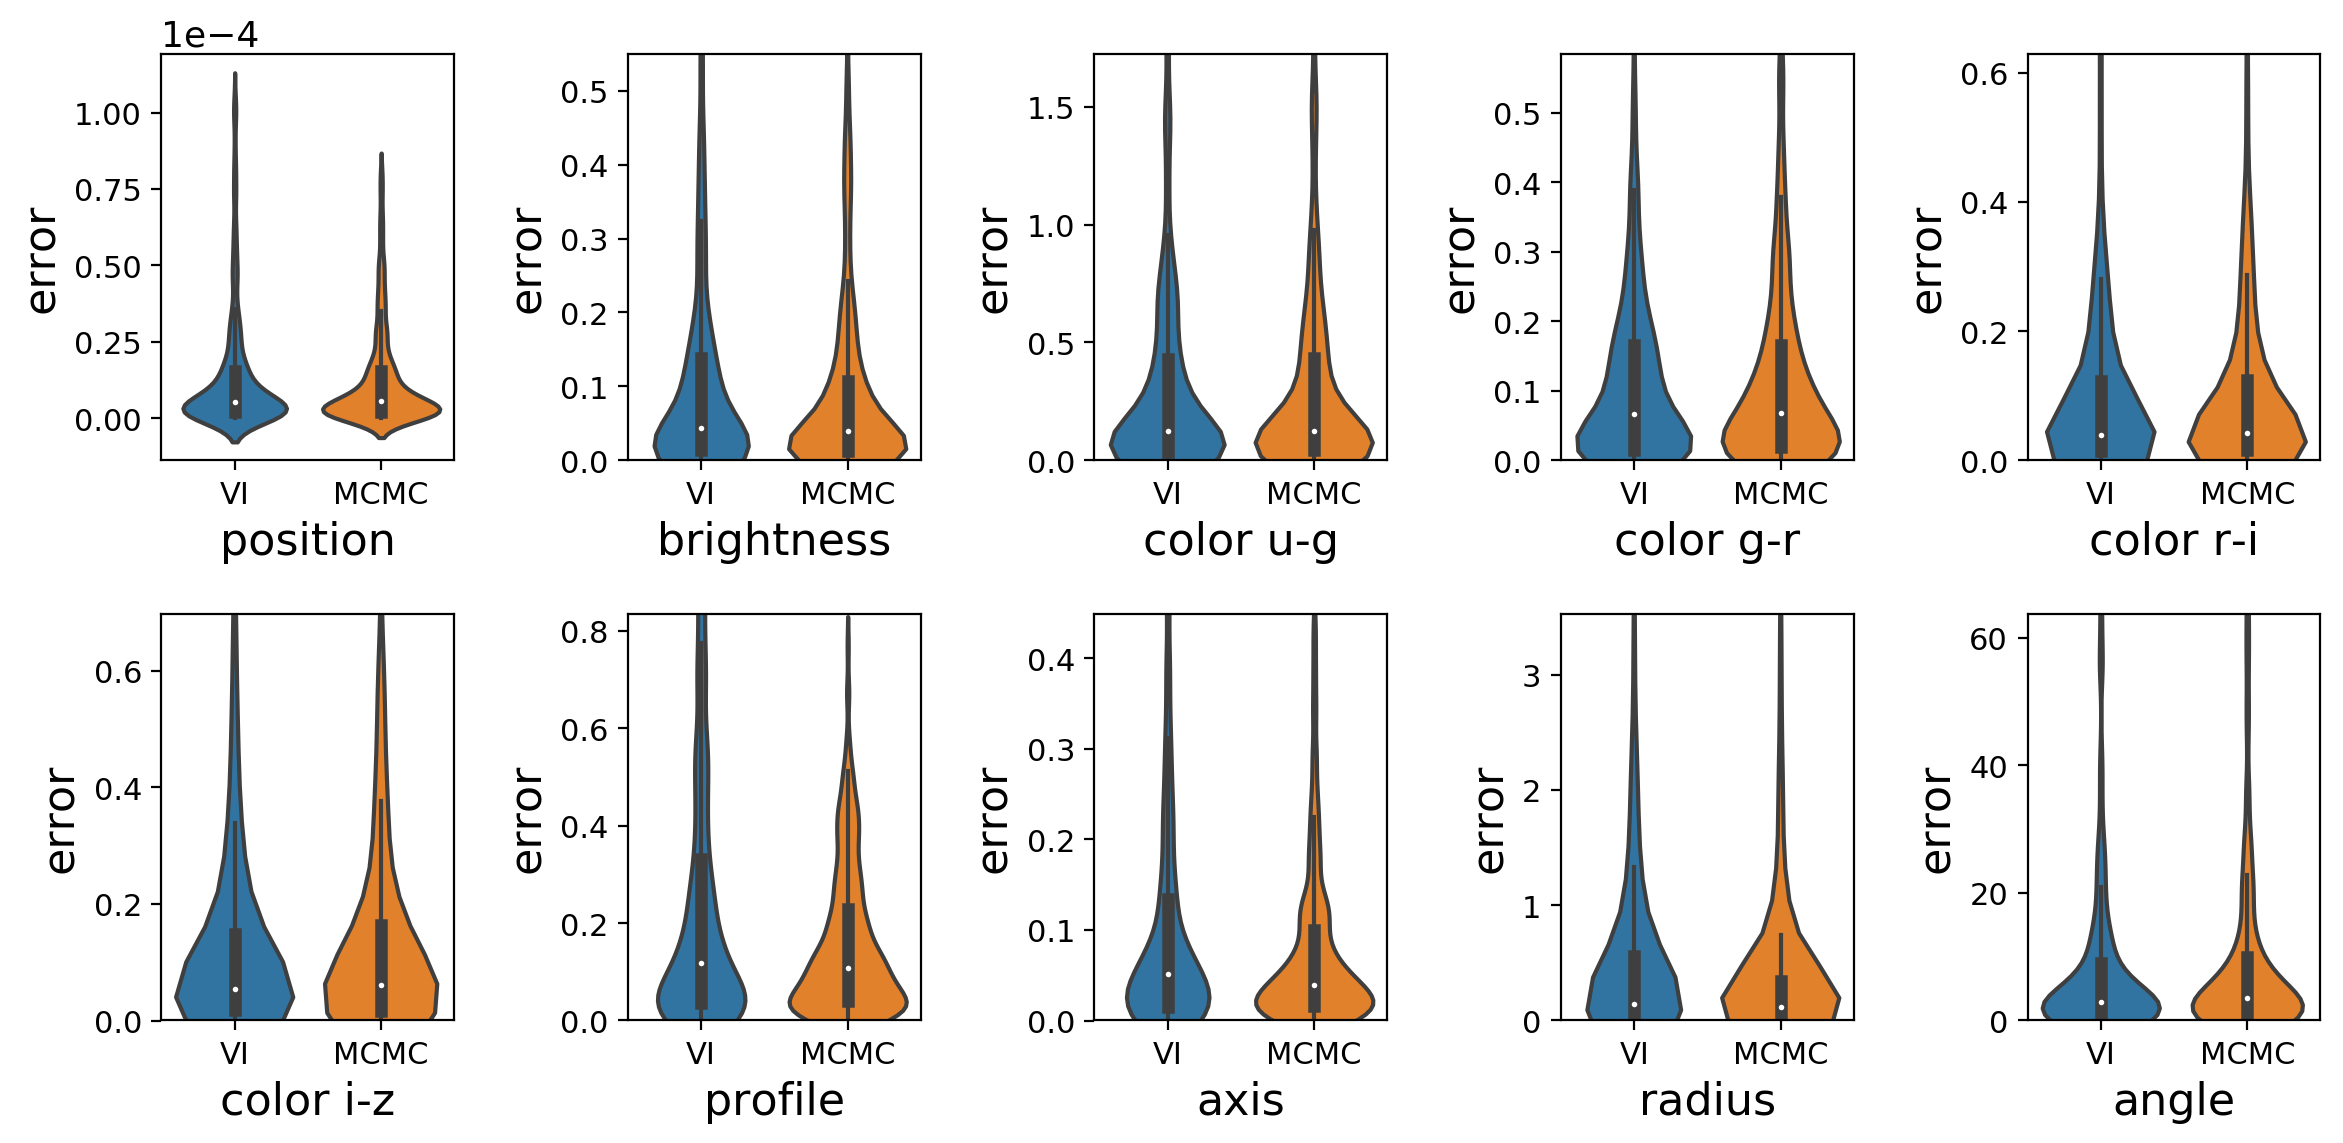}
  \caption{Comparison of error distribution on synthetic data.
  \textbf{Lower is better.}
  ``Direction'' is error, in pixels, for the directions of the light sources'
  centers.
  ``Flux'' measures the reference band (r-band) flux.
  ``Colors'' are ratios of magnitudes in consecutive bands.
  ``Profile'' is a proportion indicating whether a galaxy is de Vaucouleurs
  or exponential.
  ``Axis ratio'' is the ratio between the lengths of a galaxy's minor and
  major axes.
  ``Radius'' is the half-light radius of a galaxy in pixels.
  ``Angle'' is the orientation of a galaxy in degrees.}
\label{err-synth}
\end{figure}

%----- stripe 82 error results ----
\begin{figure}
  \centering
  \includegraphics[width=\linewidth]{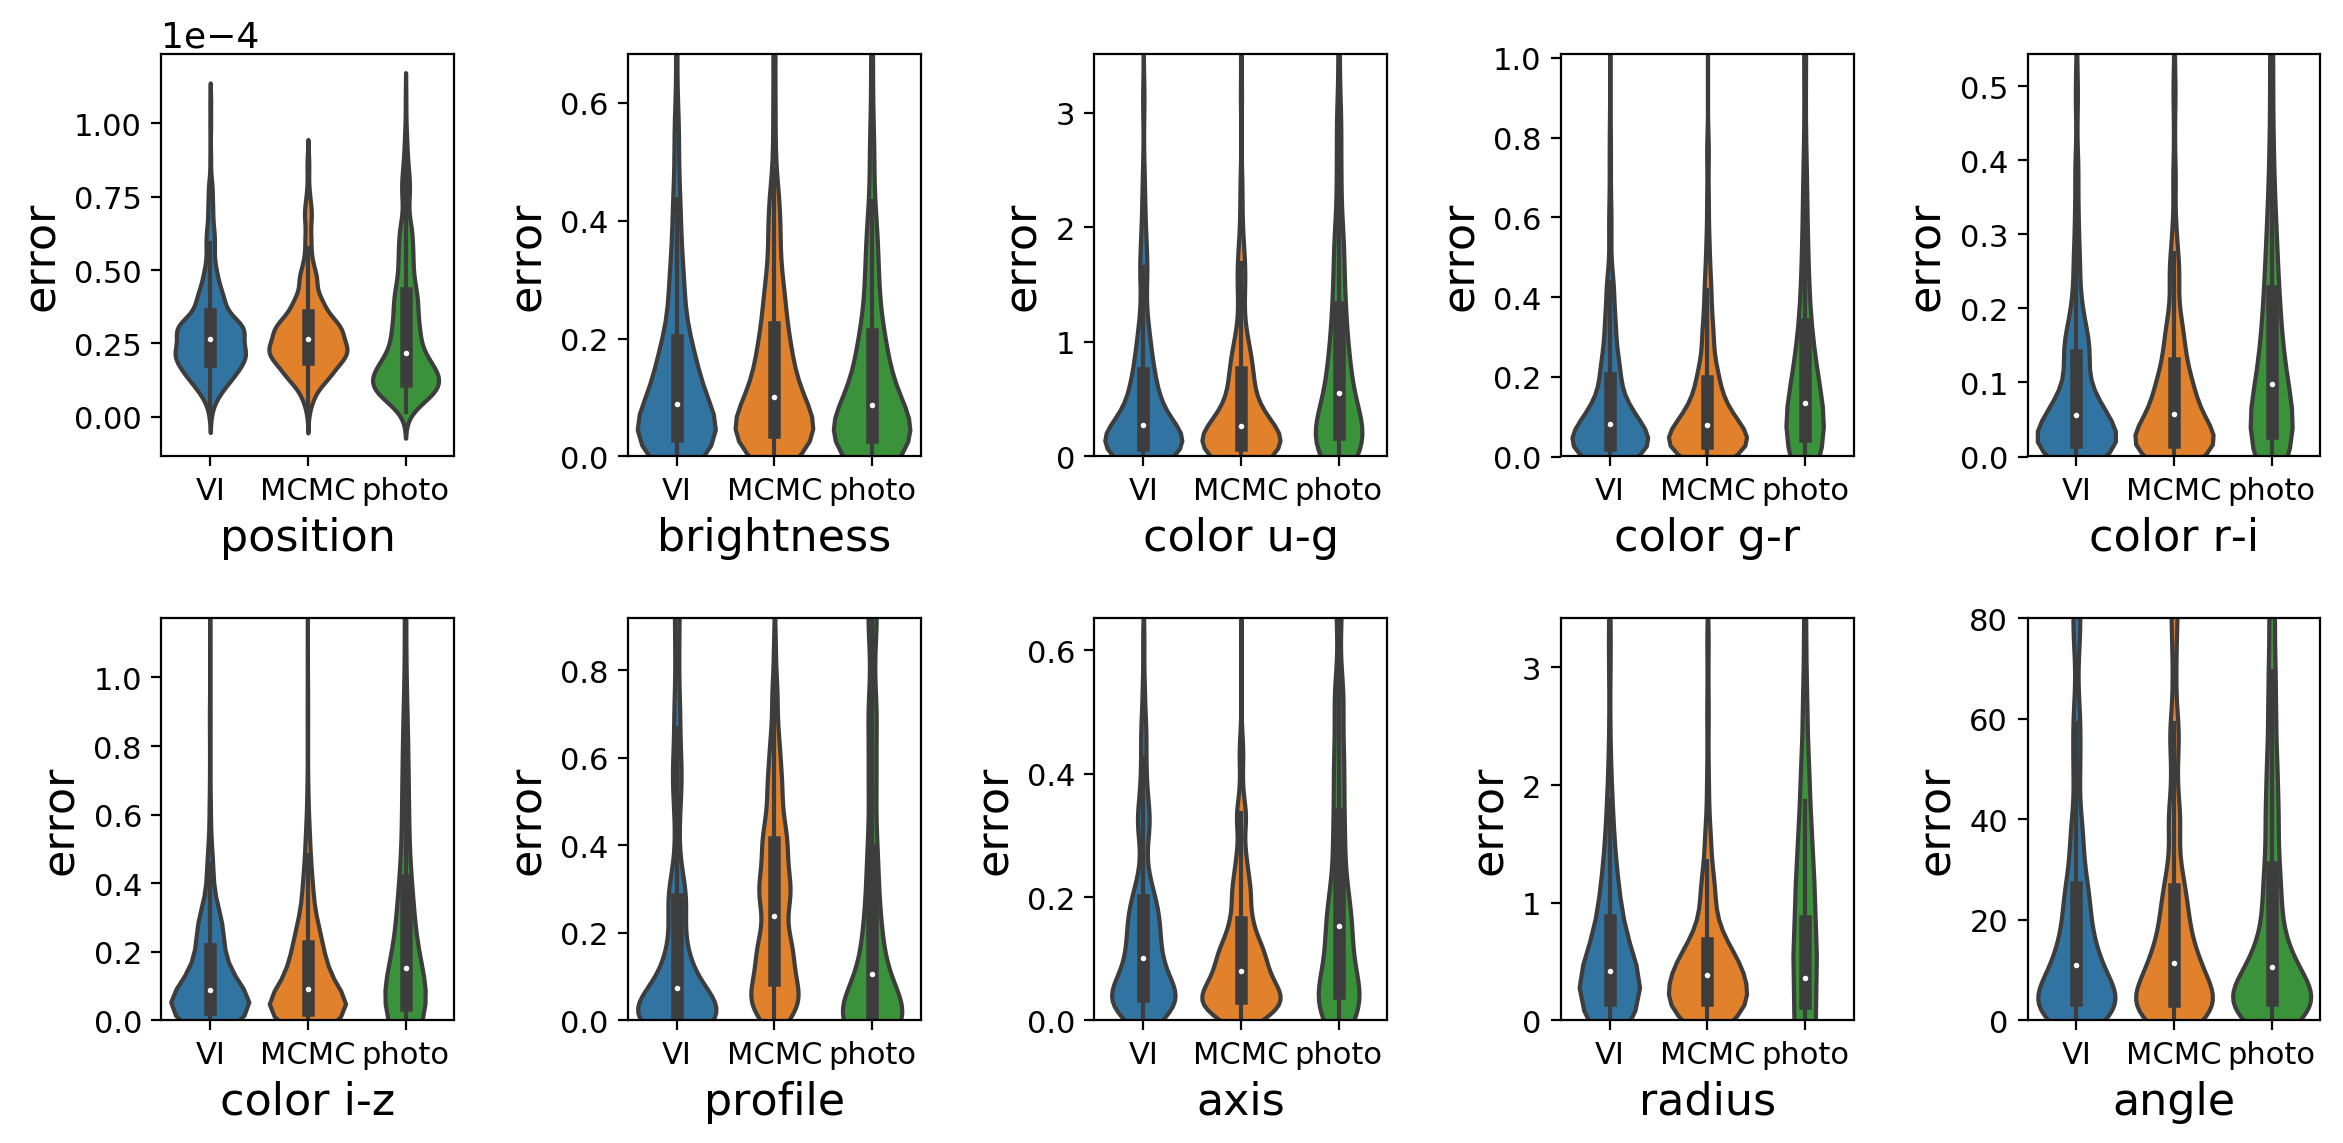}
  \caption{Comparison of absolute error distributions on Stripe 82 data.}
\label{err-real}
\end{figure}
